# Supplementary material for: Mixed-state quantum anomaly and multipartite entanglement
Source: arXiv:2401.17357 source file (2024-11-29)

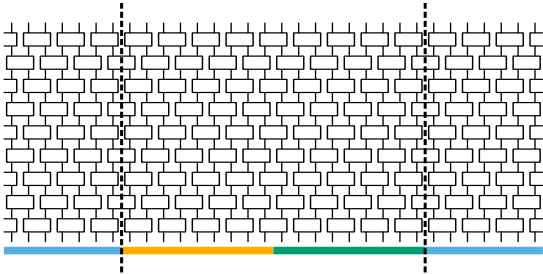

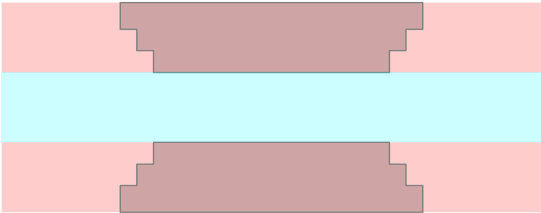

Supplement: Supplementary file 1 [file local_unitary_surgery_appendix.pdf]
